# Supplementary material for: How to cleave cubic perovskite oxides
Source: arXiv:2408.08996 ancillary file (2024-08-16)
Supplement: Supplementary file 1 [file Supplement_HowToCleaveCubicPerovskiteOxides.pdf]

# SUPPLEMENTAL MATERIAL

## How to cleave cubic perovskite oxides

Igor Sokolović,[1,*] Michael Schmid,[1] Ulrike Diebold,[1] and Martin Setvín[1,2]

[1] *Institute of Applied Physics, TU Wien, Wiedner Hauptstrasse 8-10/134, 1040 Vienna, Austria*

[2] *Department of Surface and Plasma Science, Faculty of Mathematics and Physics, Charles University, V Holešovičkách 2, 180 00 Prague 8, Czech Republic*

**CONTENTS**

SM1. Methods 2

SM2. The pre-straining procedure 3

SM3. Cleaving thick $SrTiO_3$ crystals 5

SM4. Additional details on the cleaving of the $SrTiO_3$(001), $KTaO_3$(001), and $BaTiO_3$(001) 6

References 6

* Corresponding author: igor.sokolovic@unileoben.ac.at

## SM1. METHODS

For Fig. 1 of the main text, the cleaving device was custom made and home-built out of stainless steel, with more details laid out below in section SM2. The $SrTiO_3$ single crystal was purchased in a custom shape, which is discussed further when elaborating the properties of used cubic perovskites in section SM4. The modeling, the calculations, and the results were performed and visualized using the Fusion 360 software by Autodesk® ; more details in section SM3

For Figs. 2a–c of the main text, the SEM images were acquired using FEI Quanta 200F measurement setup, evacuated to a nominal vacuum of $1 \times 10^{-5}$ mbar. An Everhart–Thornley detector was used for the detection of secondary electrons. All surfaces imaged with SEM were acquired with an incident electron energy of 5 kV. SEM imaging was performed at the USTEM facility of the TU Wien. The two halves of the cleaved $SrTiO_3(001)$ surface shown in Fig. 2 of the main text were exposed to ambient conditions during the transfer from a UHV laboratory to the USTEM facility. In fact, one of the surfaces was exposed to ambient conditions more than a month, yet the SEM contrast still showed clear contrast differences, consistent with the distribution of the two terminations on a cleaved $SrTiO_3(001)$ surface.

For Fig. 2d of the main text, atomically resolved noncontact atomic force microscopy images of the two terminations on the cleaved $SrTiO_3(001)$ surface were acquired in a low-temperature Omicron qPlus AFM/STM head. The measurement head is located in UHV with base pressure below $10^{-11}$ mbar, and the measurements were performed at a temperature of 4.8 K. The nc-AFM tips were prepared by electrochemically etching tungsten tips and subsequent cleaning *in situ* by self-sputtering with $Ar^+$ ions [1]. The tips were attached to custom design qPlus tuning forks with a separate wire for the tunneling current [2], at the end of the oscillating prong. The qPlus sensors had a resonance frequency of 28 kHz and a Q-factor of ≈50000. The deflection signal of the oscillating prong was detected and measured using a cryogenic differential preamplifier [3]. Low mechanical noise during measurement was achieved by decoupling the entire chamber from the surrounding vibrations by suspending it on bungee cords [4].

For Fig. 3 of the main text, the optical photographs were acquired using the Olympus SZX12 microscope with an attached Olympus E-330. All images were acquired with a similar orientation of the incident light. The orientation of the cleaved surfaces is indicated in the very first panel, and is consistent on all other photographs. Each $SrTiO_3$ single crystal in Fig. 3 of the main text was 2 mm thick.

For Fig. 4 of the main text, tapping-mode ambient AFM images were acquired using an Agilent 550 scanning probe microscope. The AFM cantilevers used were OLYMPUS OMCL-AC240TS with an reflective Al coating at the backside to reflect the incoming infrared laser used for detecting the deflection of the cantilever.

## SM2. THE PRE-STRAINING PROCEDURE

Bulk-truncated $SrTiO_3(001)$ surfaces can be systematically and reproducibly achieved with the pre-straining device depicted in Fig. 1a in the main text. The good practices and common pitfalls regarding the construction details and the practical details of the pre-straining and cleaving procedure for single crystals using this device are presented here using $SrTiO_3$ as an example.

Figure 1a in the main text shows detailed photographs of the cleaving device. The cleaving device consists of two identical clamping sets that squeeze a single crystal at the top and the bottom, such that they create a double-decker structure visible in photographs II and II in Fig. 1a in the main text. Both, the bottom and the top set of clamps, consist of a large and a small jaw; they are connected by two M2 screws; the small clamp has a 2 mm diameter holes, while the large clamp has M2 threads at the corresponding positions. All jaws must be well polished, in order to apply uniform pressure to the single crystal. The optimum polishing for the large clamp was found to be at a $5^\circ$ angle at the face that will be touching the single crystal, such that the contact between the crystal and the jaws occurs in a very small area at the edge of the jaws. This is depicted in the drawing V of Fig. 1a in the main text. Both the top and the bottom large jaws were polished with $\approx 5^\circ$ angle such that the contact occurs only at the very small region, at the border of the volume where the cleavage should occur. The quality of alignment is easily checked by placing the cleaving device, with a single crystal mounted inside, in front of a light source and verifying that the contact between the large jaw and a single crystal is as small as possible, as depicted in the photograph III in Fig. 1a in the main text. Each large jaw is fixed to its corresponding flag-type sample holder plates via an M2 screw. The small jaws on the other hand are free to move, and are fixed to the large jaws by two M2 screws and applying pressure to the single crystal. For this reason, small jaws should not be polished with the same inclination as the large clamps, but perpendicular to the axes of the M2 clamping screws. When a crystal is clamped between the large and the small jaws, it will be lifted from the sample plate it previously stood on, as seen in the zoom-in photograph marked with "2" in Fig. 1a in the main text. This occurs due to the application of force to a single crystal, which inclines it towards the small clamp by an angle that cannot exceed the $\approx 5^\circ$ polishing angle of the large clamp.

The bottom and the top set of clamps are held together only *via* the squeezed single crystal between them. After a single crystal has been sufficiently squeezed by the bottom set of clamps, a small spacer needs to be inserted on top of the bottom part so that the top part can be mounted such that there is a small gap between the two parts of the double-decker construction. This gap (visible in the photograph marked III in Fig. 1a in the main text) defines the crystal volume that is directly subjected to the uniaxial "squeezing" stress, and this is where the single crystal will eventually cleave. This separation can be easily achieved by placing two pieces of spacer sheet (0.1 mm thick) at each side of the clamped single crystal, and resting the top set of clamps on top of them. After tightening the top set of clamps, they will not be parallel to the bottom set of clamps any more, but instead incline due to the inclination of the already squeezed single crystal along the large jaws.

The clamping procedure requires experience and caution. Proper alignment of the bottom set of clamps is crucial for ensuring a high-quality cleavage. Initially, a single crystal is placed on the sample plate close to the already fixed large bottom clamp, resting on the bottom face — in the case of $SrTiO_3$, this was chosen to be the $(00\bar{1})$ face. The single crystal is then squeezed by turning the M2 screws which drive the small clamp towards the single crystal. It is imperative that the gradual squeezing occurs in a way as equal as possible through the two M2 screws: if one side of the small bottom clamp is prematurely squeezing the crystal while the other side is still not in contact, the single crystal will be squeezed inhomogeneously. Once the small bottom jaw is securely in contact with the single crystal, as parallel as possible, the M2 screws need to be tightened with an appropriate torque. The exact value of torque necessary to ensure high-quality cleavage was not evaluated, but it is close to the force that would lead to damaging the screws. If one of the screws is tightened too much, an imbalance between the sides of the single crystal can induce spontaneous fracturing. Even if the two M2 screws are tightened "simultaneously" up to the plastic deformation of the screws, large stress will crush the single crystal at the contact point with the clamps and destroy it. When the clamping with the bottom set of clamps is completed, tightening the top set of clamps is more challenging because this is the final step of preparation after which the sample is ready for cleaving. In other words, one has to take care not to induce a cleavage when mounting the top set of clamps. The complete cleaving device with the mounted sample is then transfered to UHV with caution, to avoid accidental cleaving during transport, insertion into the loadlock transfer arm, or insertion into a sample storage. The properly pre-squeezed crystals cleave with very little applied force.

Any material of choice for constructing the clamps can be used: so far we have tested clamps made out of stainless steel, molybdenum, and aluminum-zinc alloy. Experience shows that stainless steel clamps are by far the best. A successful cleavage will leave an imprint on the steel clamps in the contact area with the sample due to the local plastic deformation following the application of stress during screw tightening. This imprint can also serve as an indicator of how strongly the sample was clamped, what the contact area with the sample was, and whether the clamping was properly parallel with respect to the face of the sample that was oriented towards the small clamp (normal to (001) in

the case of $SrTiO_3$). After each cleaving, all clamps have to be re-polished at those faces that were in contact with the sample in order to remove the material plastically deformed, visible as an imprint. This step usually requires very little polishing as the imprint into the stainless steel is not deep, *i.e.* gentle sandpaper is preferred for this step (we typically use grit 800, followed by 1200). After polishing, the entire device requires cleaning prior to the next mounting, and the stainless steel construction offers the possibility of boiling in 20% diluted $HNO_3$ for efficient cleaning. The only downside of the stainless steel cleaving device is that is cannot withstand high temperatures that would be used for investigating the effect of annealing on the cleaved surfaces, in which case molybdenum is the material of choice.

The sample is finally cleaved in UHV by pushing the ear of the flag-type sample holder plate that is a part of the top half of the double-decker shown in Fig. 1a in the main text, using the UHV wobble stick. The bottom of the flag-type sample holder plates is preferably held inside the manipulator of the UHV chamber, or the sample storage in UHV, whichever is sturdier. After cleaving, the bottom set of clamps with one half of the cleaved crystal remains in this position, while the top set of clamps and the remaining half of the cleaved crystal is held in the wobble stick by the ear of the flag-type sample holder plate. Therefore, a succesfull cleavage creates two well-defined $SrTiO_3(001)$ surfaces, one held by the bottom set of clamps and the other held by the top set of clamps. Since both are mounted on standardized flag-type sample holder plates, either or both can be used for subsequent measurements in UHV. Both the bottom and the top set of clamps are keeping the two halves of a cleaved single crystal firm enough that AFM/STM measurements can be performed at low temperatures, without the interference of mechanical vibrations.

When a $SrTiO_3$ single crystal sample is properly pre-strained outside of UHV, very little force is necessary to cleave it with a wobble stick in UHV. The rule of thumb is that the easier the $SrTiO_3$ sample cleaves. In some cases, when the force required for cleaving was higher than simply touching the top part of the device, in which case a successful cleavage could also be achieved, albeit with lower probability. When a single crystal requires a lot of force to cleave, it is better to stop the cleaving, and instead take the cleaving device outside of UHV for adjustment of the clamps and the application of higher strain to the single crystal. In the case of $SrTiO_3$, if a lot of force is required for cleaving, the sample will usually simply fracture conchoidally once sufficient force is applied.

The small size of the cleaving device limits the size of single crystals used for cleaving. The entire cleaving device is situated on a $18{\times}15\,\mathrm{mm}^2$ flag-type sample holder plate that is suited for a typical UHV system, namely for the wobble sticks, transfer arms, manipulators, sample storages and the low-temperature AFM/STM head. A cleaving device with M2 screws (Fig. 1a in the main text) is close to the upper size limit for such UHV systems; a cleaving device with M3 screws would be already too large to fit the standard flag-type sample holder. The same considerations apply to the size of the $SrTiO_3$ single crystals designed for cleaving: their height is limited to $\approx$8 mm, but their width could be, in principle, as large as 5 mm and still fit into this cleaving device. However, cleaving 5 mm thick single crystals with this setup is challenging because only a limited amount of strain can be achieved using the M2 screws. If the cleaving device was not limited in size to fit on a standard flag-type sample holder plate, larger clamps and larger diameter screws could be used – these could apply higher forces and potentially enable succesfull cleaving arbitrarily thick samples. Experience shows that application of such larger clamps outside of UHV does enable easier cleaving.

## SM3. CLEAVING THICK $SrTiO_3$ CRYSTALS

Due to the limited amount of strain that can be applied with a small cleaving device depicted in Fig. 1a in the main text, 1 mm thick samples cleave better than thicker crystals. They commonly cleave very well, with the majority of the surface flat and atomically well-defined. However, many area-averaging experimental methods require a large surface area due to the finite irradiation spot size, or the limited acceptance are of the energy analyzers. This plays a role in in x-ray photoelectron spectroscopy (XPS), low-energy electron diffraction (LEED), low-energy ion scattering spectroscopy (ISS), or synchrotron radiation in angle-resolved photoemission spectroscopy (ARPES), for example. For spot sizes larger than 1 mm, cleaving $SrTiO_3$ crystals thicker than 1 mm is necessary, but the limited amount of applicable strain poses a challenge.

Cleaving 2 mm thick $SrTiO_3$ samples can also be performed successfully using the small cleaving device presented in Fig. 1a in the main text. All $SrTiO_3(001)$ surfaces in Figs. 2 and 3 of the main text were obtained by cleaving 2 mm thick crystals. Experience shows that cleaving these crystals is not as straightforward as cleaving thin crystals. Namely, the strain applied prior to cleaving with the small cleaving device has to be properly engineered for successful cleaving of the thick crystal. This was further investigated by simulating and comparing the strain distribution during cleaving in both, 1 mm and 2 mm thick samples in Fig. 1c of the main text. The pre-straining was simulated by applying 2 kN/m torque to each of the four M2 screws used for squeezing.

Clamping with M2 screws tensioned with 2 kN/m is efficient for 1 mm thick crystals, depicted in the left panel of Fig. 1c of the main text, since the strain is distributed across the crystal volume along the [110] direction. For samples that are 2 mm thick, the application of the same amount of strain was calculated to result in the highest strain distribution on the [001] edges of a single crystal that are closest to the M2 threads. This happens becaue the smaller (and thinner) jaw tends to bend under the load, therefore most of the strain is applied at the edges of the rectangular crystal. This results in an undesirable strain distribution, with low strain in the center. Additionally, small pieces may get chipped off at the edges of the crystal. These problems are worst for thick crystals, where higher forces are needed than for thin ones. The strain distribution during clamping can be engineered to efficiently span the crystal volume of 2 mm thick crystals by removing (polishing off) [001] edges that would otherwise experience the highest strain, as shown in the strain simulation in the right panel of Fig. 1c in the main text. After removal of the sharp [001] edges on thicker crystals, they can be successfully cleaved, albeit the relative percentage of well-cleaved surface areas compared to conchoidally fractured surface is commonly lower compared to thinner crystals. Nevertheless, the total surface area that is well-cleaved on 2 mm thick samples cleaved this way is much larger than what would be available on 1 mm thick samples, and therefore enables reliable measurements with the area-averaging techniques. Cleaving even thicker $SrTiO_3$ single crystals would be desirable, but requires larger cleaving devices that do not fit into the typical low-temperature STM/AFM measurement heads of the UHV chambers with standardized $18\times15\,mm^2$ flag-type sample holder plates.

## SM4. ADDITIONAL DETAILS ON THE CLEAVING OF THE $SrTiO_3$(001), $KTaO_3$(001), AND $BaTiO_3$(001)

Cleaved, bulk-terminated strontium titanate $SrTiO_3$(001) surfaces were obtained by cleaving $SrTiO_3$ single crystals through the procedure described in this work. $SrTiO_3$(001) surfaces presented in the main text in Fig. 2 and Fig. 3 were obtained by cleaving single crystals with orientation shown in Fig. 4a of the main text: these $SrTiO_3$ crystals with a $3{\times}7\,\mathrm{mm}^2$ large (110) face, $2\times7\,\mathrm{mm}^2$ large ($1\bar{1}0$) face, and $3\times7\,\mathrm{mm}^2$ large (001) face were bought from CrysTec GmbH, SurfaceNet GmbH, and MaTecK GmbH. Differently-oriented and differently-sized $SrTiO_3$(001) surfaces are shown only in the second panel of Fig. 4 of the main text: These custom shaped $SrTiO_3$ crystals with a $2{\times}8\,\mathrm{mm}^2$ large (100) face, $2\times8\,\mathrm{mm}^2$ large (010) face, and $2\times2\,\mathrm{mm}^2$ large (001) face were bought from MaTecK GmbH. All $SrTiO_3$ samples presented in the main text had the same level of nominal Nb doping of 0.5 at%. $SrTiO_3$ was routinely cleaved both in ambient and UHV to achieve some of the results presented here. Majority of samples were cleaved at room temperature.

The $KTaO_3$ samples cleaved in Fig. 4 of the main text were bought from Stanford Advanced Materials in a custom shape with a $3{\times}8\,\mathrm{mm}^2$ large (100) face, $1{\times}8\,\mathrm{mm}^2$ large (010) face, and $1\times2\,\mathrm{mm}^2$ large (001) face. The $KTaO_3$ samples were nominally undoped. The $KTaO_3$(001) surface in Fig. 4c of the main text was obtained by cleaving in ambient, at room temperature.

The $BaTiO_3$ samples cleaved in Fig. 4d of the main text were bought from MaTecK GmbH in a custom shape with a $3{\times}3\,\mathrm{mm}^2$ large (100) face, $3{\times}8\,\mathrm{mm}^2$ large (010) face, and $3\times3\,\mathrm{mm}^2$ large (001) face. The $KTaO_3$ samples were nominally undoped. The $BaTiO_3$(001) surface in Fig. 4d of the main text was obtained by cleaving in ambient, at room temperature.

[1] M. Setvín, J. Javorský, D. Turčinková, I. Matolínová, P. Sobotík, P. Kocán, and I. Ošt'ádal, Ultrasharp tungsten tips—characterization and nondestructive cleaning, Ultramicroscopy **113**, 152 (2012).
[2] F. J. Giessibl, Sensor for noncontact profiling of a surface (2013), US Patent 8,393,009.
[3] F. Huber and F. J. Giessibl, Low noise current preamplifier for qPlus sensor deflection signal detection in atomic force microscopy at room and low temperatures, Rev. of Sci. Instr. **88**, 073702 (2017).
[4] M. Schmid, M. Setvín, and U. Diebold, Device for suspending a load in a vibration-insulated manner (2019), US Patent App. 16/327,528.
